# Supplementary material for: Motion Primitives Planning For Center-Articulated Vehicles
Source: arXiv:2405.17127 source file (2024-10-04)
Supplement: Supplementary file 1 [file 06_appendix.tex]

\section*{APPENDIX}
